# Supplementary material for: Magnon scattering in the transport coefficients of CoFe alloys
Source: arXiv:1802.01038 source file (2018-02-03)
Supplement: Supplementary file 1 [file Supplement_ver8small.pdf]

# Supplementary Material for Magnon scattering in the transport coefficients of CoFe alloys

S. Srichandan<sup>1</sup>, S. Wimmer<sup>2</sup>, M. Kronseder<sup>1</sup>, H. Ebert<sup>2</sup>, C.H. Back<sup>1</sup>, and C. Strunk<sup>1</sup>

<sup>1</sup>*Institute of Experimental and Applied Physics, University of Regensburg, D-93040, Germany and*

<sup>2</sup>*Department of Chemistry, Physical Chemistry, Ludwig-Maximilians University, Munich, D-81377, Germany*

(Dated: January 16, 2018)

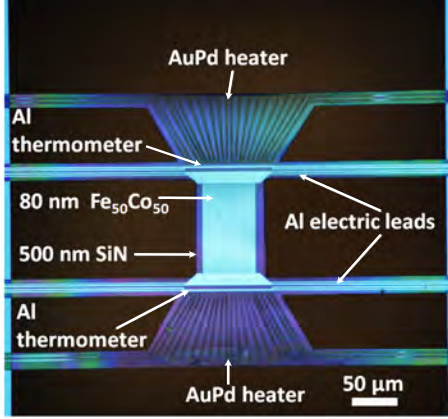

FIG. S1. Optical image of a typical device with an allocation of the different elements.

## SCHEMATIC OF A TYPICAL DEVICE

Figure S1 shows an optical image of the central region of a typical suspended microcalorimeter for the measurement of the transport coefficients as seen from the top. The central rectangle constitutes the 80 nm thick  $\text{Co}_{50}\text{Fe}_{50}$  film. The 40 nm thick  $\text{Au}_{60}\text{Pd}_{40}$  meander heaters are placed onto trapezoidal islands at both ends of the bridge. Thermometers and electrical leads are made of 50 nm thick Al. The suspended 500 nm thick SiN membrane appears as purple background, while the etched regions are seen as dark empty areas.

## MORE DETAILS ABOUT THE RESISITIVITY

We decompose the total resistivity into a residual and a  $T$ -dependent part:  $\rho = \rho_0 + \Delta\rho(T)$ . In Figure S2 the residual resistivity  $\rho_0(x_{\text{Co}})$  of all five samples at  $T = 26$  K is plotted. It is maximal near  $x_{\text{Co}} = 0.20$  then decreases monotonically with addition of Co. Our data are well in line with earlier data on bulk samples [1–3]. The solid green line has been calculated within the Kubo formalism accounting for chemical disorder via the CPA alloy theory (see Sec. below). It systematically underestimates our experimental data and for  $x_{\text{Co}} < 0.4$  also those of Ref. 1.

Taking into account chemical disorder only,  $\rho_0(x_{\text{Co}})$  is reproduced qualitatively by our model calculations. When compared to pure Fe and Co, but also to bulk al-

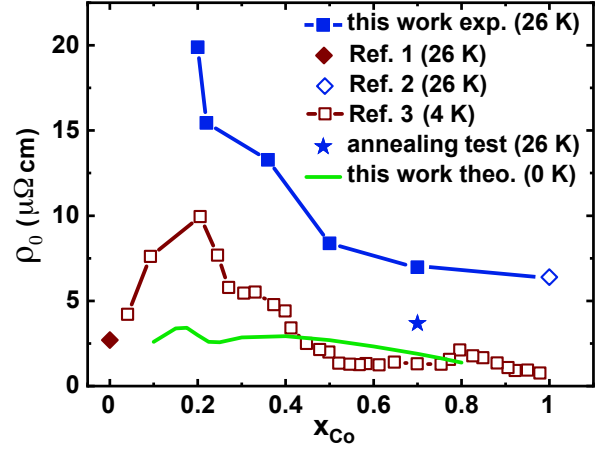

FIG. S2. Residual resistivity  $\rho(x_{\text{Co}})$  from this work at 26 K (filled squares), after annealing (filled star), from literature (20 nm Fe at 26 K (filled diamond [1]), 53 nm Co (open diamond [2]), and bulk CoFe at 4.2 K (open squares [3]), and the calculated contribution of chemical disorder at 0 K (line).

loy samples, the values of  $\rho_0$  are significantly higher than expected for purely chemical disorder, i.e., a perfect bcc lattice with a random distribution of Fe and Co atom on the lattice sites. This indicates a rather high degree of additional structural disorder in our films. In order to test this assumption we performed an annealing test at  $400^\circ\text{C}$  for 5 minutes with a film with  $x_{\text{Co}} = 0.7$ . The annealing led to a significant drop of  $\rho$  from  $6.94 \mu\Omega \text{ cm}$  to  $3.68 \mu\Omega \text{ cm}$  at 26 K [blue star in Fig. S2].

Next we discuss the separation of phonon and magnon contributions to  $\Delta\rho(T)$ . According to the analysis of Ref. [4, 5] the magnon contribution  $\rho_{\text{mag}}$  becomes sizable only above  $T \simeq 100$  K. We first determine the phonon contribution by fitting the measured  $\rho(T)$  to a Bloch-Wilson (BW) function

$$\Delta\rho_{\text{phon}}(T) = \alpha_{\text{ep}} \left( \frac{T}{\Theta_R} \right)^3 \int_0^{\Theta_R/T} \frac{x^3 dx}{(e^x - 1)(1 - e^{-x})} \quad (\text{S1})$$

from 26 K up to 100 K, where the magnon contribution is expected to be very small. The free parameters  $\alpha_{\text{ep}}$  and  $\Theta_R$  represent the electron-phonon coupling constant and a characteristic phonon temperature  $\Theta_R$ , respectively. We extract  $\Theta_R \simeq 260 - 280$  K from these fits, which is about 25% smaller than  $\Theta_{\text{Debye}}$  of pure Fe or Co [6].

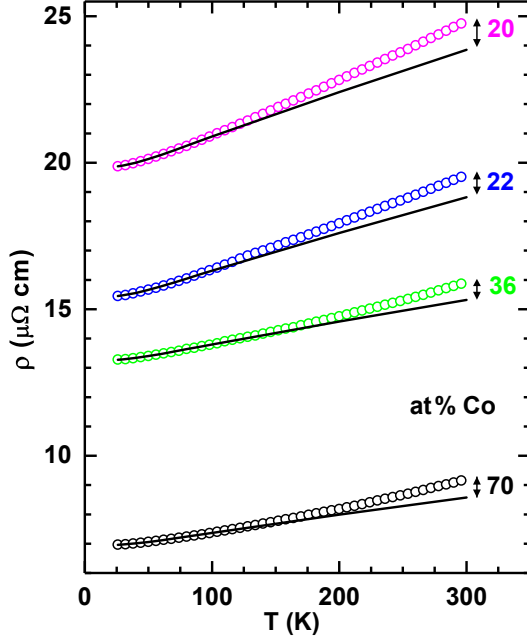

FIG. S3. Resistivity data and Bloch-Wilson fits (see main text) from 26 K to 100 K and extrapolated to 296 K (lines) on measured data (open circles) as a function of temperature at varying  $\Theta_R$  for (a) 20 % Co, (b) 22 % Co, (c) 36 % Co and (d) 70 % Co.  $\rho_{\text{mag}}$  is shown as a double headed arrow at the highest temperature.

Such a discrepancy between the characteristic temperatures extracted from equilibrium and transport quantities is not surprising, as the Debye model characterizes the phonon spectrum only very roughly.

Figure S3 shows the results for films with 20, 22, 36 and 70 % Co. The disorder in our films is also reflected in the temperature dependence  $\rho(296 \text{ K}) - \rho(26 \text{ K})$ ;  $\rho$  changes by  $2 \sim 5 \mu\Omega \text{ cm}$  between 26 and 296 K which is about half of the values  $6.2 \mu\Omega \text{ cm}$  and  $10.4 \mu\Omega \text{ cm}$  for bulk Co and Fe, respectively. A similar reduction of the phonon resistivity in thin films has been observed earlier [7]. Extrapolating to 300 K we can evaluate the magnon contribution  $\rho_{\text{mag}}(T)$  (marked by double-headed arrows) by subtracting the BW-fit (lines) from the measured  $\rho(T)$ . The magnon contribution is at most 6.5% of  $\rho$  at room temperature for  $x_{\text{Co}} = 0.20$ , and thus only a fraction of the phonon contribution.

#### DETAILS OF TEP MEASUREMENT

As explained in the main text, the thermopower is determined from the ratio of measured thermovoltage  $\Delta V_{\text{th}}$  and the temperature difference of  $\Delta T$ . In particular at lower bath temperatures  $T$  it is important to assure that  $\Delta V_{\text{th}}$  depends linearly on  $\Delta T$ . At a given base temperature, the thermovoltage  $\Delta V_{\text{th}}$  and the temperature dif-

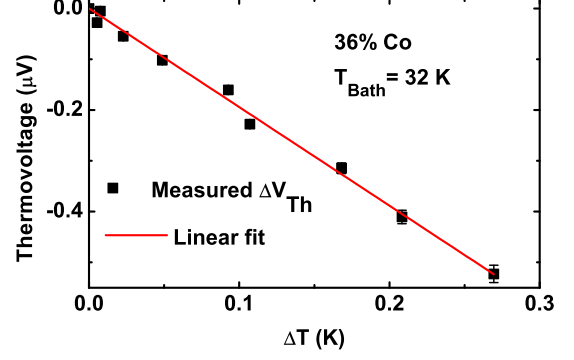

FIG. S4. Measured thermovoltage as a function of  $\Delta T$  for a film with 36% Co at temperature of 32 K is shown as black squares and the red line represents the linear fit of the data with zero intercept.

ference  $\Delta T$  between the islands is measured for a series of applied heater powers. Figure S4 shows a typical plot of  $\Delta V_{\text{th}}$  vs.  $\Delta T$  at 32 K while maintaining  $\Delta T$  smaller than  $\simeq 1\%$  of the corresponding bath temperature.

The decomposition of the total thermopower into  $S_{\text{Mott}}$  and  $S_{\text{mag}}$  according to Eq. 2 has been explained in the main text. Fig. S5 is an illustration of such a decomposition for a film with  $x_{\text{Co}}=0.7$ . The measured data is shown as black dots to which Equation 2 is fitted as a red line in the temperature range above 100 K. The contributions  $S_{\text{Mott}} \propto T$  and  $S_{\text{mag}} \propto T^{3/2}$ , are parameterized by the respective prefactors  $S'_{\text{Mott}}$  and  $S'_{\text{mag}}$ . The resulting individual contributions are shown as squares and triangles, respectively. Note that the curvature in the raw data occurs predominantly at low temperature. This evidences the necessity of a non-linear term in this

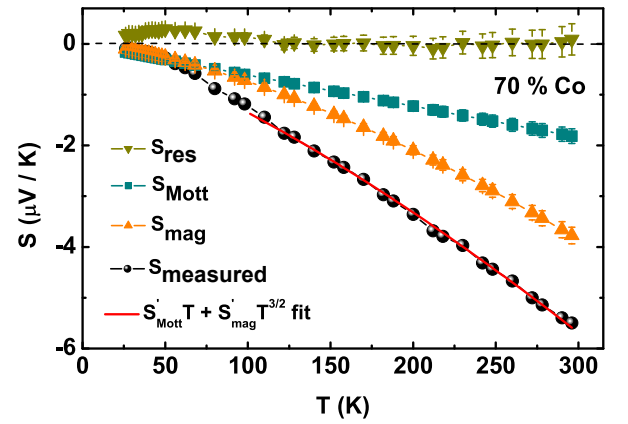

FIG. S5. Total measured thermopower (black dots) and corresponding fit function (red line) for a film with  $x_{\text{Co}}=0.7$ . The squares, triangles and the inverted triangles represent the  $S_{\text{Mott}}$ ,  $S_{\text{mag}}$  and  $S_{\text{Res}}$  respectively.

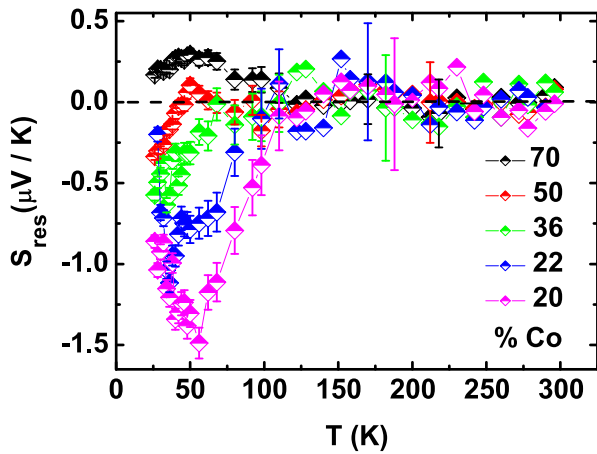

FIG. S6.  $S_{\text{res}}$  for all five  $\text{Co}_x\text{Fe}_{1-x}$  films vs temperature from 50 K-296 K. The numbers at the right indicate Co concentration.

regime, where the Sommerfeld expansion for the diffusion TEP is still valid.

In Figure S6 we show the small residual contribution to the TEP that remains after subtraction of the Mott-like and magnon drag contributions. For films in single bcc phase, i.e., films with  $x_{\text{Co}}=0.20$  and  $0.22$ , we find small dips are reminiscent of the phonon-drag effect. For films in mixed phase, the contribution from in-elastic scattering could produce such peaks. Additionally the diffusion thermopower of Al contacts is included in  $S_{\text{res}}$ , it is possible that residues of a phonon-drag peak in the thermopower of the Al leads provide a positive contribution to the peak structures below 100 K.

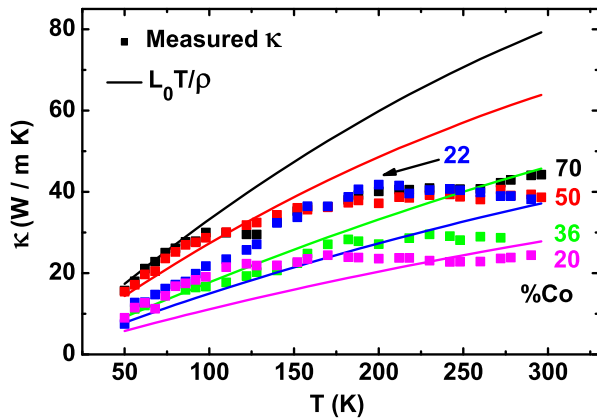

FIG. S7. Thermal conductivity  $\kappa$  for all 5  $\text{Co}_x\text{Fe}_{1-x}$  films vs temperature graph from 50 K-296 K is shown as squares. The numbers at the right indicate Co concentration. The lines represent the Wiedemann-Franz expectation value  $\kappa_e$ .

## THERMAL CONDUCTIVITY OF CoFe ALLOYS

Figure S7 shows the measured thermal conductivity  $\kappa$  of the five CoFe films as a function of temperature. For comparison we plot the electronic contribution to  $\kappa_{\text{el}}$  as calculated from the measured resistivity using the Wiedemann-Franz law:  $\kappa_{\text{el}} = 2.45 \times 10^{-8} \text{ W}\Omega/\text{K}^2 \times T/\rho$  (lines in Fig. S7). Only for the films with lower Co concentrations (20% and 22%), the difference  $\kappa - \kappa_{\text{el}}$  is positive (see Fig. 3(c) in the main text) and can be assigned to a phonon contribution (at lower  $T$ ) or to a phonon/magnon scattering contribution (at higher  $T$ ) to the thermal conductivity. The magnon contribution to  $\kappa$  is usually visible below a few K only, when the phonon contribution is already negligible.

## DETAILS OF THE FIRST-PRINCIPLES CALCULATIONS

The electronic structure of the bcc  $\text{Co}_x\text{Fe}_{1-x}$  alloys has been determined using the spin-polarised relativistic Korringa-Kohn-Rostoker band structure method [8, 9] as implemented in the Munich SPR-KKR program package [10]. Chemical disorder is treated within the Coherent Potential Approximation (CPA) [11, 12]. For the entire concentration range considered here, the bcc structure has been assumed. At selected intermediate concentrations (30, 40, 50, 60, 70 at% Co) calculations have been performed for the fcc phase as well, assuming the same volume per atom as in the bcc structure of the same composition. Lattice parameters have been taken from literature [13] and interpolated appropriately for *intermediate* [14] concentrations. For the self-consistent determination of spin-polarised ground-state potentials the fully relativistic version of the program has been used. The exchange and correlation part is treated within the Local Spin-Density Approximation (LSDA) using the parametrisation of Vosko *et al.* [15]. All calculations were done in the Atomic Sphere Approximation (ASA) [16] for the potential shape.

The symmetric and antisymmetric parts of the electric conductivity tensor have been determined within Kubo's linear response framework using the Kubo-Greenwood and -Středa formulae, respectively [17–24]. These are derived in the athermal limit of the Kubo-Bastin equation [25, 26] and have been shown to yield numerically identical results for the type of systems treated here (cubic transition metals) in the limit  $T \rightarrow 0$  [27]. Inclusion of the so-called vertex corrections (VC) [20, 28] is necessary to correct for improper averaging within the Coherent Potential Approximation (CPA) when dealing with products of Green's functions. For calculating electric, thermoelectric, and thermal transport properties

at finite electronic temperatures, the generalized Mott formula [29–33] and related expressions for the charge-charge (cc), charge-heat (cq), and heat-heat (qq) current correlation functions or response coefficients

$$L_{ij}^{cc}(T) = -\frac{1}{|e|} \int dE \sigma_{ij}^{cc}(E) \left( -\frac{\partial f(E,T)}{\partial E} \right) \quad (\text{S2})$$

$$L_{ij}^{cq}(T) = -\frac{1}{|e|} \int dE \sigma_{ij}^{cc}(E) \left( -\frac{\partial f(E,T)}{\partial E} \right) (E - E_F) \quad (\text{S3})$$

$$L_{ij}^{qq}(T) = -\frac{1}{|e|} \int dE \sigma_{ij}^{cc}(E) \left( -\frac{\partial f(E,T)}{\partial E} \right) (E - E_F)^2 \quad (\text{S4})$$

in terms of the energy-dependent electric conductivity  $\sigma_{ij}^{cc}(E)$  have been used. Here  $T$  is the (electronic) temperature, entering via the Fermi-Dirac distribution  $f(E, T)$ ,  $e$  is the elementary charge, and the integral over real energies  $E$  contains the product of the energy-dependent electrical conductivity  $\sigma_{ij}^{cc}(E)$  with a kernel consisting of the (negative) energy derivative of  $f(E, T)$  and a factor of  $(E - E_F)^n$ , where  $n$  equals the number of heat currents  $q$  involved and  $E_F$  is the Fermi energy. The Alloy Analogy Model [34] for temperature-induced vibrational and fluctuational disorder has been applied using calculated  $M(T)$  data from Kakehashi and Hosohata [35] as input for the latter. For intermediate concentrations where results are not available in Ref. 35 linear interpolations between fits to

$$M(T)/M(0) = (1 - (T/T_C)^\alpha)^\beta \quad (\text{S5})$$

have been performed.

### CALCULATED RESISTIVITY INCLUDING VARIOUS SOURCES OF DISORDER

The isotropic residual resistivity  $\rho_{\text{iso}} = (2\rho_{xx} + \rho_{zz})/3$  is shown as a function of temperature for the exemplary case of  $\text{Co}_{0.50}\text{Fe}_{0.50}$  in Fig. S8. Temperature is treated here on the level of the alloy-analogy model accounting for either lattice displacements only (red squares), transverse spin fluctuations only (green triangles), or both combined (blue circles). The total result including both sources of disorder simultaneously on the level of the Green function is obviously dominated by the vibrational disorder contribution and the two effects are nearly additive following Matthiessen's rule. As discussed in the main text, the as-prepared samples show a considerable amount of structural disorder. To compensate for this, a finite and constant imaginary part of the complex energy  $z$  was chosen for a quantitative agreement at low temperature with the experimental data shown as black diamonds. Corresponding results are given in magenta

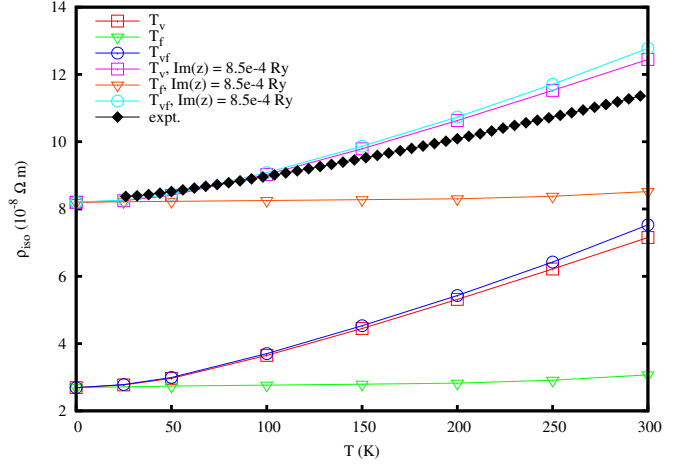

FIG. S8. Calculated isotropic resistivity  $\rho_{\text{iso}} = (2\rho_{xx} + \rho_{zz})/3$  in  $\text{Co}_{0.50}\text{Fe}_{0.50}$  accounting for lattice disorder ( $T_v$ , red), transverse spin disorder ( $T_f$ , green), and both combined ( $T_{vf}$ , blue). In purple, orange and cyan corresponding results are shown including in addition an energy-independent finite imaginary part of the complex energy,  $\Im(z) = 8.5 \cdot 10^{-4}$  Ry, mimicking structural disorder in the experiment, results of which are shown in black.

( $T_v$ ), orange ( $T_f$ ), and cyan ( $T_{vf}$ ). The finite imaginary part, corresponding to an additional decrease of the electronic lifetime, leads to an overall increase of the resistivity without major modification of the temperature dependence. Considering in addition the effect of a modified Fermi-Dirac statistics by means of Eq. S2 leads only to minor changes at higher  $T$  (not shown).

### CALCULATED SEEBECK COEFFICIENT

The Seebeck or thermoelectric tensor, expressing the ratio of charge transport due to a temperature gradient versus that in response to an electric field, is obtained from Eqs. (S2) and (S3) as

$$\underline{S} = -\frac{1}{eT} (\underline{L}^{cc})^{-1} \underline{L}^{cq} = \underline{\sigma}^{-1} \underline{\alpha} = \begin{pmatrix} S_{xx} & S_{xy} & 0 \\ -S_{xy} & S_{xx} & 0 \\ 0 & 0 & S_{zz} \end{pmatrix} = \begin{pmatrix} \frac{\sigma_{xx}\alpha_{xx} + \sigma_{xy}\alpha_{xy}}{\sigma_{xx}^2 + \sigma_{xy}^2} & \frac{\sigma_{xx}\alpha_{xy} - \sigma_{xy}\alpha_{xx}}{\sigma_{xx}^2 + \sigma_{xy}^2} & 0 \\ -\frac{\sigma_{xx}\alpha_{xy} - \sigma_{xy}\alpha_{xx}}{\sigma_{xx}^2 + \sigma_{xy}^2} & \frac{\sigma_{xx}\alpha_{xx} + \sigma_{xy}\alpha_{xy}}{\sigma_{xx}^2 + \sigma_{xy}^2} & 0 \\ 0 & 0 & \frac{\alpha_{zz}}{\sigma_{zz}} \end{pmatrix}, \quad (\text{S6})$$

where  $\underline{\sigma} = -e\underline{L}^{cc}$  is the electrical conductivity tensor and  $\underline{\alpha} = -\frac{1}{T}\underline{L}^{cq}$  is the Nernst conductivity tensor. In the limit of  $T \rightarrow 0$  K the energy integrals in Eqs. (S2) and (S3) transform via the Sommerfeld expansion into the well-known Mott formula.

When comparing to experimental results the isotropic value  $S_{\text{iso}} = \frac{2}{3}S_{xx} + \frac{1}{3}S_{zz}$ , i.e., one third of the tensor in

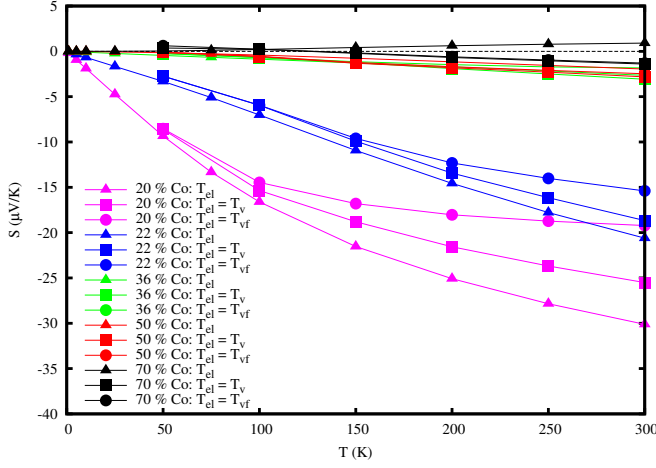

FIG. S9. Calculated thermoelectric power for bcc  $\text{Co}_x\text{Fe}_{1-x}$  treating temperature either only on the level of the Fermi-Dirac distribution (*electronic temperature*,  $T_{el}$ , triangles), including in addition vibrational disorder ( $T_v$ , squares), and including both, vibrational and spin-fluctuation disorder ( $T_{vf}$ , circles).

Eq. (S6) is used. Neglecting off-diagonal contributions as in  $S_{ii} = -\frac{1}{eT} L_{ii}^{cq}/L_{ii}^{cc}$  leads however, for the systems and conditions considered in this work, only to minor differences, since  $L_{ij}^{AB} \ll L_{ii}^{AB}$  holds for both  $\underline{L}^{cc}$  and  $\underline{L}^{cq}$ . Additional contributions arising from direct and inverse spin Nernst and Hall effects, such as the spin Nernst magnetothermopower [36], are neglected in this work due to their vanishingly small size.

Figure S9 shows results for bcc  $\text{Co}_x\text{Fe}_{1-x}$  with  $x = 0.20, 0.22, 0.36, 0.50$ , and  $0.70$  accounting for chemical disorder only ( $T_{el}$ ), including, by means of the alloy-analogy model, the effect of lattice displacements alone ( $T_v$ ) or in combination with transverse spin fluctuations ( $T_{vf}$ ). The effect of the additional temperature-dependent disorder apparently leads to a reduction of the TEP for low Co content (as well as to an increased curvature), to minor enhancement for intermediate  $x_{\text{Co}}$  (0.36 and 0.50), and to sign change for  $x_{\text{Co}} = 0.70$ . The importance of spin disorder decreases with increasing Co content, consistent with the decrease of the Curie temperature and simultaneous increase of the slope of the  $M(T)$  curves [35] entering the calculations as input.

### ENERGY-DEPENDENT CONDUCTIVITY

The theoretical results for the energy-dependent conductivity are shown in Fig. S10 taking account the chemical disorder only (0 K) and including vibrational disorder corresponding to a temperature of  $T_v = 100$ , K. At higher  $T$  the rather sharp step in  $\sigma(E)$  qualitatively explains the rather large values of the Mott-like contribution to the TEP at low  $x_{\text{Co}}$ . The step width is comparable to the

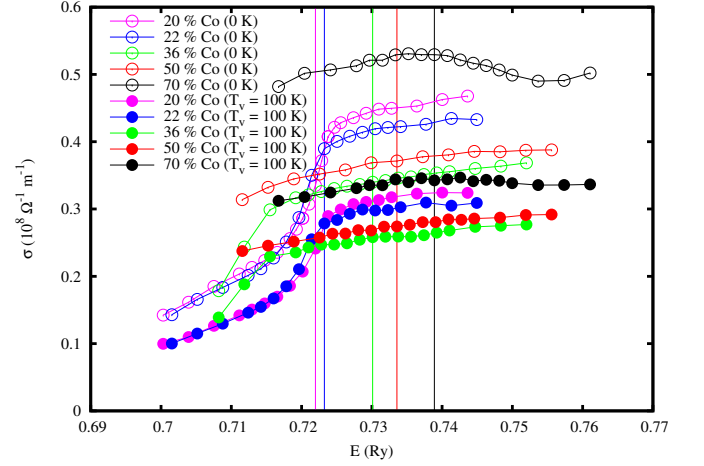

FIG. S10. Energy dependence of the conductivity of bcc  $\text{Co}_x\text{Fe}_{1-x}$  at zero temperature (empty symbols) and  $T_v = 100$  K (full symbols). The vertical lines indicate the positions of the respective Fermi levels at  $T = 0$  K.

temperature so that the leading term in the Sommerfeld expansion is not sufficient to calculate the TEP – at higher temperatures this leads to a curvature in the  $T$ -dependence of Fig. 2d in the main manuscript. The temperature dependent contributions of vibrational and spin disorder (not shown) tend to smear the step, in addition to a reduced overall magnitude. On the other hand,  $\sigma(E)$  is rather flat on the high energy side, which leads to much lower values of the TEP than observed in the experiment for the Mott-like contribution.

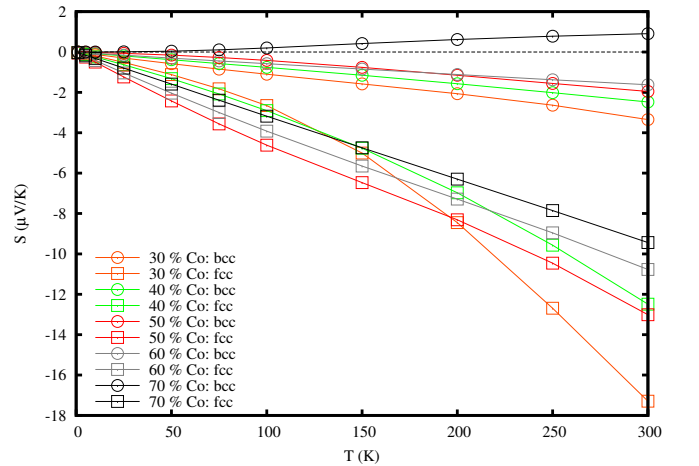

FIG. S11. Calculated electronic contribution to the Seebeck coefficient in bulk bcc and fcc  $\text{Co}_x\text{Fe}_{1-x}$  for  $x = 0.30, 0.40, 0.50, 0.60$ , and  $0.70$ .

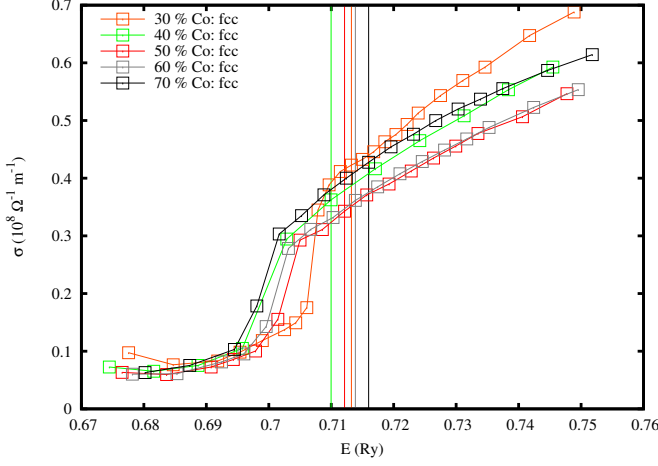

FIG. S12. Energy dependence of the conductivity of fcc  $\text{Co}_x\text{Fe}_{1-x}$  at zero temperature. The vertical lines indicate the positions of the respective Fermi levels.

### THERMOELECTRIC POWER IN THE FCC PHASE

This discrepancy may result from fcc precipitations which appear at higher  $x_{\text{Co}}$  in the characterization. Such precipitation are also consistent with the low phonon contribution in the thermal conductivity. For this reason we also calculated the TEP for the fcc structure. The results are plotted in Fig. S11, and show that for the fcc lattice structure significantly larger values of the TEP are found and that the curvature is opposite to that in the bcc-structure for low Co concentrations. Thus the competition between the contributions from both structures may explain the observed evolution of the TEP with Co-content at high temperatures.

The underlying energy-dependent electrical conductivities are shown in Fig S12 for  $T = 0\text{ K}$ , the Fermi levels are again indicated by the vertical lines of corresponding color. The major differences compared to the bcc curves in Fig. S10 are the pronounced, approximately linear increase of  $\sigma$  in the vicinity of the Fermi level and its relative position with respect to the step in the conductivity. The former leads to the larger Seebeck coefficient in the fcc phase for all concentrations and the latter to the negative curvature of  $\text{Co}_{0.3}\text{Fe}_{0.7}$  and  $\text{Co}_{0.4}\text{Fe}_{0.6}$ . For these two alloys with increasing temperature the step is close enough to  $E_F$  to be included in the interval for the energy integration of Eq. S3 and therefore its strong asymmetry enhances the TEP.

### CALCULATED THERMAL CONDUCTIVITY

The electronic contribution to the thermal conductivity  $\kappa$  can be calculated, assuming only elastic scattering at impurities, from the energy dependence of the

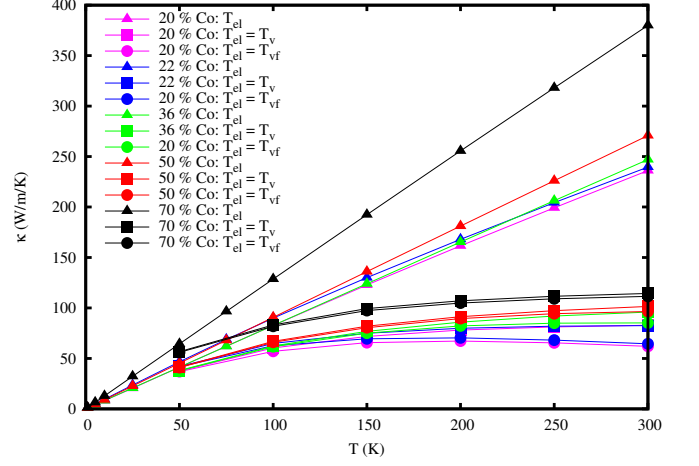

FIG. S13. Calculated electronic contribution to the thermal conductivity for bcc  $\text{Co}_x\text{Fe}_{1-x}$  treating temperature either only on the level of the Fermi-Dirac distribution (*electronic temperature*,  $T_{\text{el}}$ , triangles), including in addition vibrational disorder ( $T_v$ , squares), and including both, vibrational and spin-fluctuation disorder ( $T_{\text{vf}}$ , circles).

electrical conductivity using a generalized Mott-like expression [30, 31]. In Fig. S13 results are shown for the temperature-dependent isotropic thermal conductivity,

$$\kappa_{\text{iso}} = \frac{2}{3}\kappa_{xx} + \frac{1}{3}\kappa_{zz} \quad (\text{S7})$$

$$\text{with } \kappa_{ii} = \frac{1}{T} \left[ \underline{L}^{qq} - \frac{\underline{L}^{cq} \underline{L}^{qc}}{\underline{L}^{cc}} \right]_{ii} \quad (\text{S8})$$

$$\approx \frac{1}{T} \left( L_{ii}^{qq} - \frac{(L_{ii}^{cq})^2}{L_{ii}^{cc}} \right) \quad (\text{S9})$$

with the charge-charge, charge-heat, and heat-heat current response functions of Eqs. S2-S4 and exploiting the symmetry relations [37, 38]  $\underline{L}^{qc} = \underline{L}^{cq}$  and  $L_{ij}^{AB} = -L_{ji}^{AB}$  as well as the observation  $L_{ij}^{AB} \ll L_{ii}^{AB}$ . In the last line of Eq. S7 the contribution from off-diagonal tensor elements is neglected, the exact form of  $\underline{\kappa}$  in  $4/m\bar{m}'m'$  reads

$$\kappa_{xx} = \kappa_{yy} = \frac{1}{T} \left[ L_{xx}^{qq} - \left( \frac{L_{xx}^{cc}((L_{xx}^{cq})^2 - (L_{xy}^{cq})^2)}{(L_{xx}^{cc})^2 + (L_{xy}^{cc})^2} + \frac{2L_{xy}^{cc}L_{xx}^{cq}L_{xy}^{cq}}{(L_{xx}^{cc})^2 + (L_{xy}^{cc})^2} \right) \right] \quad (\text{S10})$$

$$\kappa_{xy} = -\kappa_{yx} = \frac{1}{T} \left[ L_{xy}^{qq} - \left( \frac{L_{xy}^{cc}((L_{xy}^{cq})^2 - (L_{xx}^{cq})^2)}{(L_{xx}^{cc})^2 + (L_{xy}^{cc})^2} + \frac{2L_{xx}^{cc}L_{xy}^{cc}L_{xx}^{cq}}{(L_{xx}^{cc})^2 + (L_{xy}^{cc})^2} \right) \right] \quad (\text{S11})$$

$$\kappa_{zz} = \frac{1}{T} \left[ L_{zz}^{qq} - \frac{(L_{zz}^{cq})^2}{L_{zz}^{cc}} \right], \quad (\text{S12})$$

leading to negligibly small corrections in case of conductive metals. The temperature dependence of the results accounting only for the electronic temperature is fairly linear and, with increasing iron content the curves fall almost on top of each other. In particular for high temperatures  $\kappa$  is strongly reduced by lattice displacements



and spin fluctuations as additional sources of disorder, the effect of the latter being again of minor importance.

## BAND STRUCTURE OF BCC $\text{Co}_x\text{Fe}_{1-x}$ ALLOYS

The transport phenomena discussed in this work show characteristic features at Co concentrations of  $\sim 20$  at%. To elucidate the composition dependence of the transport coefficients discussed in this work, the spin-projected Bloch spectral function (BSF) of the bcc alloys and their clean limits have been calculated (1<sup>st</sup> and 4<sup>th</sup> column in Fig. S14). Since the electronic contributions to the linear response properties are intimately (but not trivially) connected to the band structure, one can expect to infer a qualitative explanation for some of the concentration-dependent characteristics. As visible in Fig. S14, the overall shape of the bands is very different for the two spin channels (majority “spin-up”, left two columns, in red and minority “spin-down”, right two columns, in blue) and so is the extent as well as the  $\vec{k}$ -space position of broadening effects on the band structure. The Fermi level rises from top to bottom with growing Co content (as Fe has one electron less than Co) and at around 22% crosses the top of  $d$ -like bands of the majority channel (left) at the N point of the Brillouin zone (2<sup>nd</sup> and 3<sup>rd</sup> column in Fig. S14). This qualitatively explains the maximum of the resistivity in this concentration range, because the Fermi level is located in flat and broadened regions. For the energy dependence of the conductivity this results in the pronounced step discussed above, giving rise to distinct magnitudes and temperature dependencies for different concentrations. In the minority channel (right two columns) the bands crossing the Fermi level are predominantly of  $sp$ -character having large slopes for small cobalt concentration ( $x > 0.4$ ). At 40% Co, the Fermi level cuts through the bottom of a parabolic band in between H and N point. This should qualitatively explain the additional resistivity peak at  $x = 0.4$ . The avoided crossing at  $\sim 1/4$  of the distance between  $\Gamma$  and H point could be connected to the local minimum around 25% cobalt content, where it is passing through  $E_F$ .

---

[1] P. P. Freitas and L. Berger *Phys. Rev. B* **37**, 6079 (1988).  
 [2] M. Rubinstein, F. J. Rachford, W. W. Fuller and G. A. Prinz *Phys. Rev. B* **37**, 8689 (1988).  
 [3] J. W. C. De Vries *Thin Solid Films* **167**, 25 (1988).  
 [4] B. Raquet, M. Viret, E. Sondergard, O. Cespedes and R. Mamy *Phys. Rev. B* **66**, 024433 (2002).  
 [5] M. V. Kamalakar, A. K. Raychaudhuri, X. Wei, J. Teng and P. D. Prewett *Appl. Phys. Lett.* **95**, 013112 (2009).  
 [6] N. W. Ashcroft and N. D. Mermin, *Solid State Physics*, (Saunders College, New York 1976).  
 [7] C. Ahn, K.-H. Shin, R. Loloee, J. Bass, and W. P. Pratt, Jr. *J. Appl. Phys.* **108** 023908 (2010).

[8] H. Ebert, D. Ködderitzsch, and J. Minár, *Rep. Prog. Phys.* **74**, 096501 (2011).  
 [9] H. Ebert, J. Braun, D. Ködderitzsch, and S. Mankovsky, *Phys. Rev. B* **93**, 075145 (2016).  
 [10] *The Munich SPR-KKR package*, version 7.7, H. Ebert *et al.* <http://olymp.cup.uni-muenchen.de/ak/ebert/SPRKKR> (2017).  
 [11] P. Soven, *Phys. Rev.* **156**, 809 (1967).  
 [12] B. Velický, *Phys. Rev.* **184**, 614 (1969).  
 [13] B. Predel, “Landolt-Börnstein - Group IV Physical Chemistry,” (Springer Berlin Heidelberg, Berlin, Heidelberg, 1993), Chap. Co-Fe (Cobalt-Iron), pp. 1–13.  
 [14] That is, not for the whole range between the pure metals as in Vegard’s law.  
 [15] S. H. Vosko, L. Wilk, and M. Nusair, *Can. J. Phys.* **58**, 1200 (1980).  
 [16] O. K. Andersen, *Phys. Rev. B* **12**, 3060 (1975).  
 [17] R. Kubo, *J. Phys. Soc. Japan* **12**, 570 (1957).  
 [18] D. A. Greenwood, *Proc. Phys. Soc.* **71**, 585 (1958).  
 [19] L. Smrčka and P. Středa, *J. Phys. C: Solid State Phys.* **10**, 2153 (1977).  
 [20] W. H. Butler, *Phys. Rev. B* **31**, 3260 (1985).  
 [21] J. Banhart, R. Bernstein, J. Voigtländer, and P. Weinberger, *Solid State Commun.* **77**, 107 (1991).  
 [22] J. Banhart, H. Ebert, P. Weinberger, and J. Voigtländer, *Phys. Rev. B* **50**, 2104 (1994).  
 [23] S. Lowitzer, D. Ködderitzsch, and H. Ebert, *Phys. Rev. B* **82**, 140402(R) (2010).  
 [24] S. Lowitzer, M. Gradhand, D. Ködderitzsch, D. V. Fedorov, I. Mertig, and H. Ebert, *Phys. Rev. Lett.* **106**, 056601 (2011).  
 [25] A. Bastin, C. Lewiner, O. Betbeder-Matibet, and P. Nozieres, *J. Phys. Chem. Solids* **32**, 1811 (1971).  
 [26] A. Crépieux and P. Bruno, *Phys. Rev. B* **64**, 014416 (2001).  
 [27] D. Ködderitzsch, K. Chadova, and H. Ebert, *Phys. Rev. B* **92**, 184415 (2015).  
 [28] G. D. Mahan, *Many-Particle Physics*, 2nd ed., Physics of Solids and Liquids (Plenum Press, New York, 1993).  
 [29] M. Cutler and N. F. Mott, *Phys. Rev.* **181**, 1336 (1969).  
 [30] M. Jonson and G. D. Mahan, *Phys. Rev. B* **21**, 4223 (1980).  
 [31] M. Jonson and G. D. Mahan, *Phys. Rev. B* **42**, 9350 (1990).  
 [32] S. Wimmer, D. Ködderitzsch, K. Chadova, and H. Ebert, *Phys. Rev. B* **88**, 201108(R) (2013).  
 [33] S. Wimmer, D. Ködderitzsch, and H. Ebert, *Phys. Rev. B* **89**, 161101(R) (2014).  
 [34] H. Ebert, S. Mankovsky, K. Chadova, S. Polesya, J. Minár, and D. Ködderitzsch, *Phys. Rev. B* **91**, 165132 (2015).  
 [35] Y. Kakehashi and O. Hosohata, *Phys. Rev. B* **40**, 9080 (1989).  
 [36] S. Meyer, Y.-T. Chen, S. Wimmer, M. Althammer, T. Wimmer, R. Schlitz, S. Geprägs, H. Huebl, D. Ködderitzsch, H. Ebert, G. E. W. Bauer, R. Gross, and S. T. B. Goennenwein, *Nat. Mater.* **16**, 977 (2017).  
 [37] W. H. Kleiner, *Phys. Rev.* **142**, 318 (1966).  
 [38] M. Seemann, D. Ködderitzsch, S. Wimmer, and H. Ebert, *Phys. Rev. B* **92**, 155138 (2015).
